# Supplementary material for: (Meta-)stability and Core-Shell Dynamics of Gold Nanoclusters at Finite Temperature
Source: arXiv:1811.04438 ancillary file (2018-11-11)
Supplement: Supplementary file 1 [file supporting_information_arXiv.pdf]

# (Meta-)stability and Core-Shell Dynamics of Gold Nanoclusters at Finite Temperature Supplementary Materials

Diego Guedes-Sobrinho,[*,†] Weiqi Wang,[*,‡] Ian Hamilton,[*,¶] Juarez L. F. Da Silva,[*,†] and Luca M. Ghiringhelli[*,‡]

†*São Carlos Institute of Chemistry, University of São Paulo, PO Box 780, 13560-970, São Carlos, São Paulo, Brazil*

‡*Fritz-Haber-Institut der Max-Planck-Gesellschaft, 14195 Berlin-Dahlem, Germany*

¶*Department of Chemistry, Wilfrid Laurier University, Waterloo, N2L 3C5 Ontario, Canada*

E-mail: guedes.sobrinho.d@gmail.com; wang@fhi-berlin.mpg.de; ihamilton@wlu.ca; juarez_dasilva@iqsc.usp.br; ghiringhelli@fhi-berlin.mpg.de

Phone: +49 30 8413 4802

# I Computational details

We employed the all-electron full potential method as implemented in the Fritz-Haber-Institute - *ab initio* molecular simulations (FHI-AIMS) package,[1] from which the electrons are treated in the "atomic" scalar-relativistic approximation (atomic ZORA)[2] with atom-centered numerical atomic orbitals describing the Kohn-Sham orbitals. For all geometry relaxations, the basis set *tight-tier*2[1], as defined in the standard distribution of the FHI-AIMS package, was used. All the structures obtained by revised basin-hopping Monte Carlo (RBHMC) and the putative global-minimum cluster configurations (pGMC) form Ref. 3 were optimized using the modified Broyden–Fletcher–Goldfard–Shanno (BFGS) algorithm without symmetry constraints, to obtain the atomic forces on every atom smaller than $1.0 \times 10^{-5}$ eV/Å and using a self-consistency of $10^{-6}$ eV for the total energy. For $Au_{25}$, all the calculations were performed by using the spin-polarized mode. For $Au_{38}$ and $Au_{40}$, the spin polarized mode were investigated for few structures with non zero and zero local initial spin for the core and surface atoms separately, from which still were observed no spin density. Thus, for $Au_{38}$ and $Au_{40}$ all the calculations were performed using the non-polarized mode. Spin-orbit coupling was not considered.

The BO-MD simulations were performed with the basis set *light-tier*1[1], as defined in the standard distribution of the FHI-AIMS package. The temperature schemes for the MD runs are shown in detail in Table S1.

**Table S1 – MD schemes for the trajectories labeled by $T_1$, $T_2$, and $T_3$ for the $Au_n$ nanoclusters (n = 25, 38, and 40) and the time span for each temperature. The structures $Au_{38}$ and $Au_{40}$ as indicated by the trajectories $J_{38}$, $J_{40,1}$, and $J_{40,2}$ are the pGMC for the nanoclusters found by Jiang and Walter[3] at 0 K.**

| System | Trajectory | Temperature (Time) | Total time |
|---|---|---|---|
| $Au_n$ | $T_1$ | 400 K (50 ps) → 300 K (50 ps) | 100 ps |
| | $T_2$ | 500 K (50 ps) → 300 K (50 ps) | 100 ps |
| | $T_3$ | 600 K (50 ps) → 300 K (50 ps) | 100 ps |
| $Au_{38}$ | $J_{38}$ | 600 K (50 ps) → 300 K (50 ps) | 100 ps |
| $Au_{40}$ | $J_{40,1}$<br>$J_{40,2}$ | 600 K (50 ps) → 300 K (50 ps) | 100 ps |

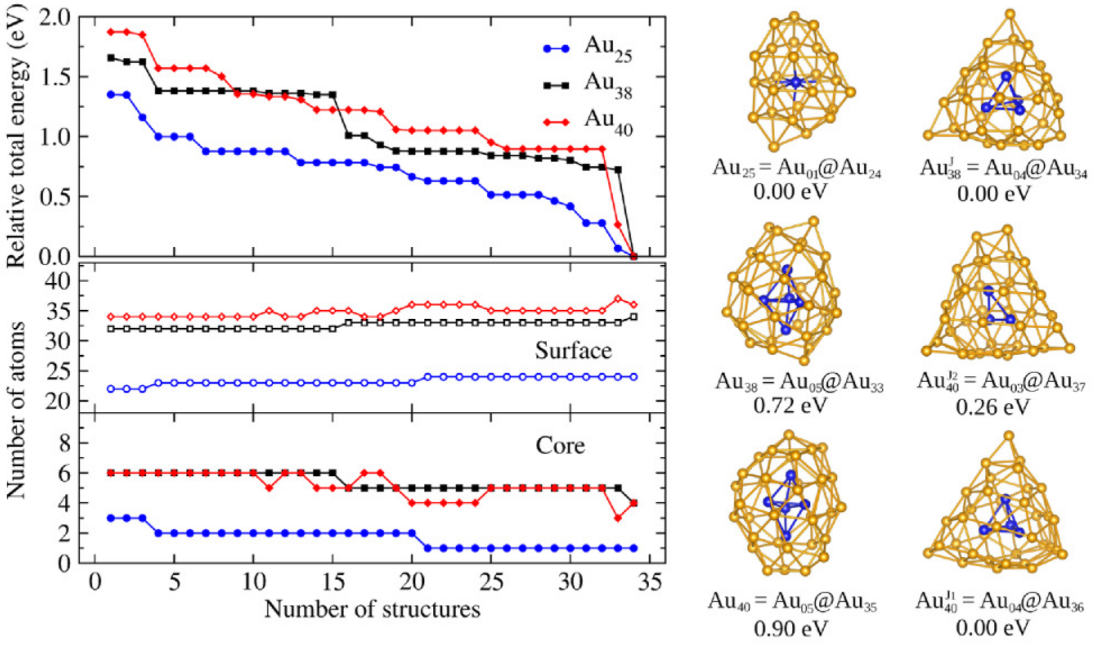

Figure S1 – On the top, relative total energies values of all structures generated using RBHMC[4] with the embedded-atom method (EAM), then locally optimized with PBE+MBD. The relative energies for $Au_{38}$ and $Au_{40}$ systems obtained with RBHMC are indicated with respect the pGMC[3], i.e., $Au_{38}{}^{J}$, $Au_{40}{}^{J1}$, and $Au_{40}{}^{J2}$. On the bottom, the number of atom for the core and surface regions are showed, matching to the relative structures above them. On the right side, the lowest energy configuration from the set of structures are represented, in which the core atoms are indicated by the blue color.

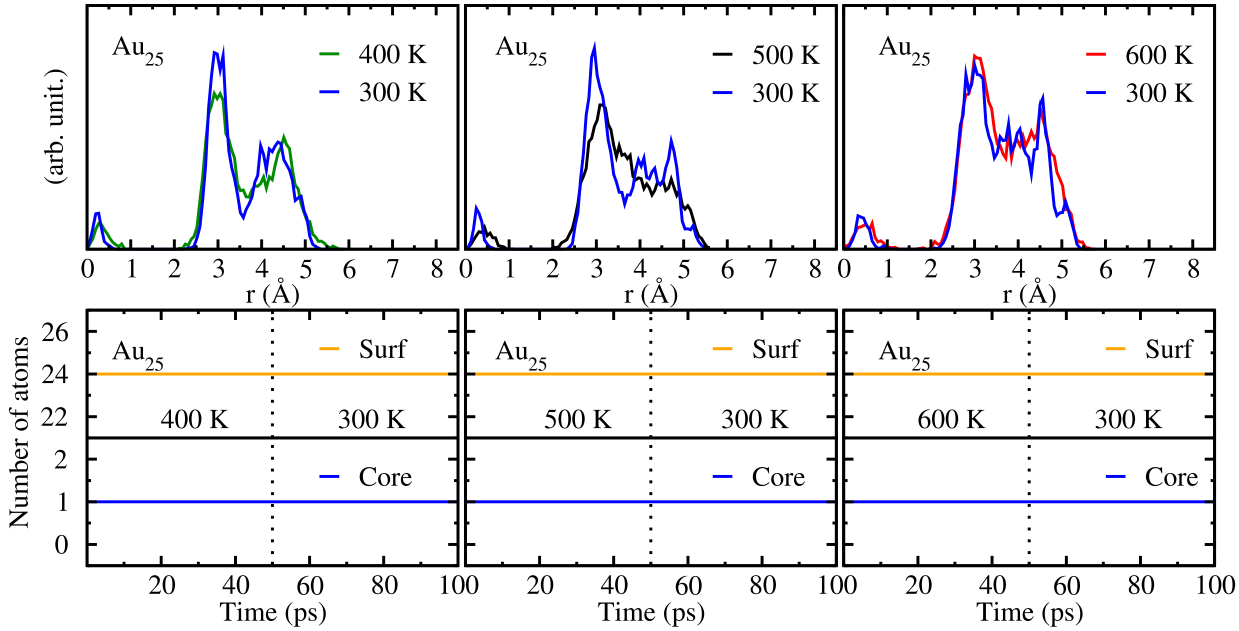

Figure S2 – Radial distribution function, $g(r)$, and number of atoms for core and surface regions, for the MD simulations at 300, 400, 500, and 600 K, starting from $Au_{25}$ obtained via RBHMC.

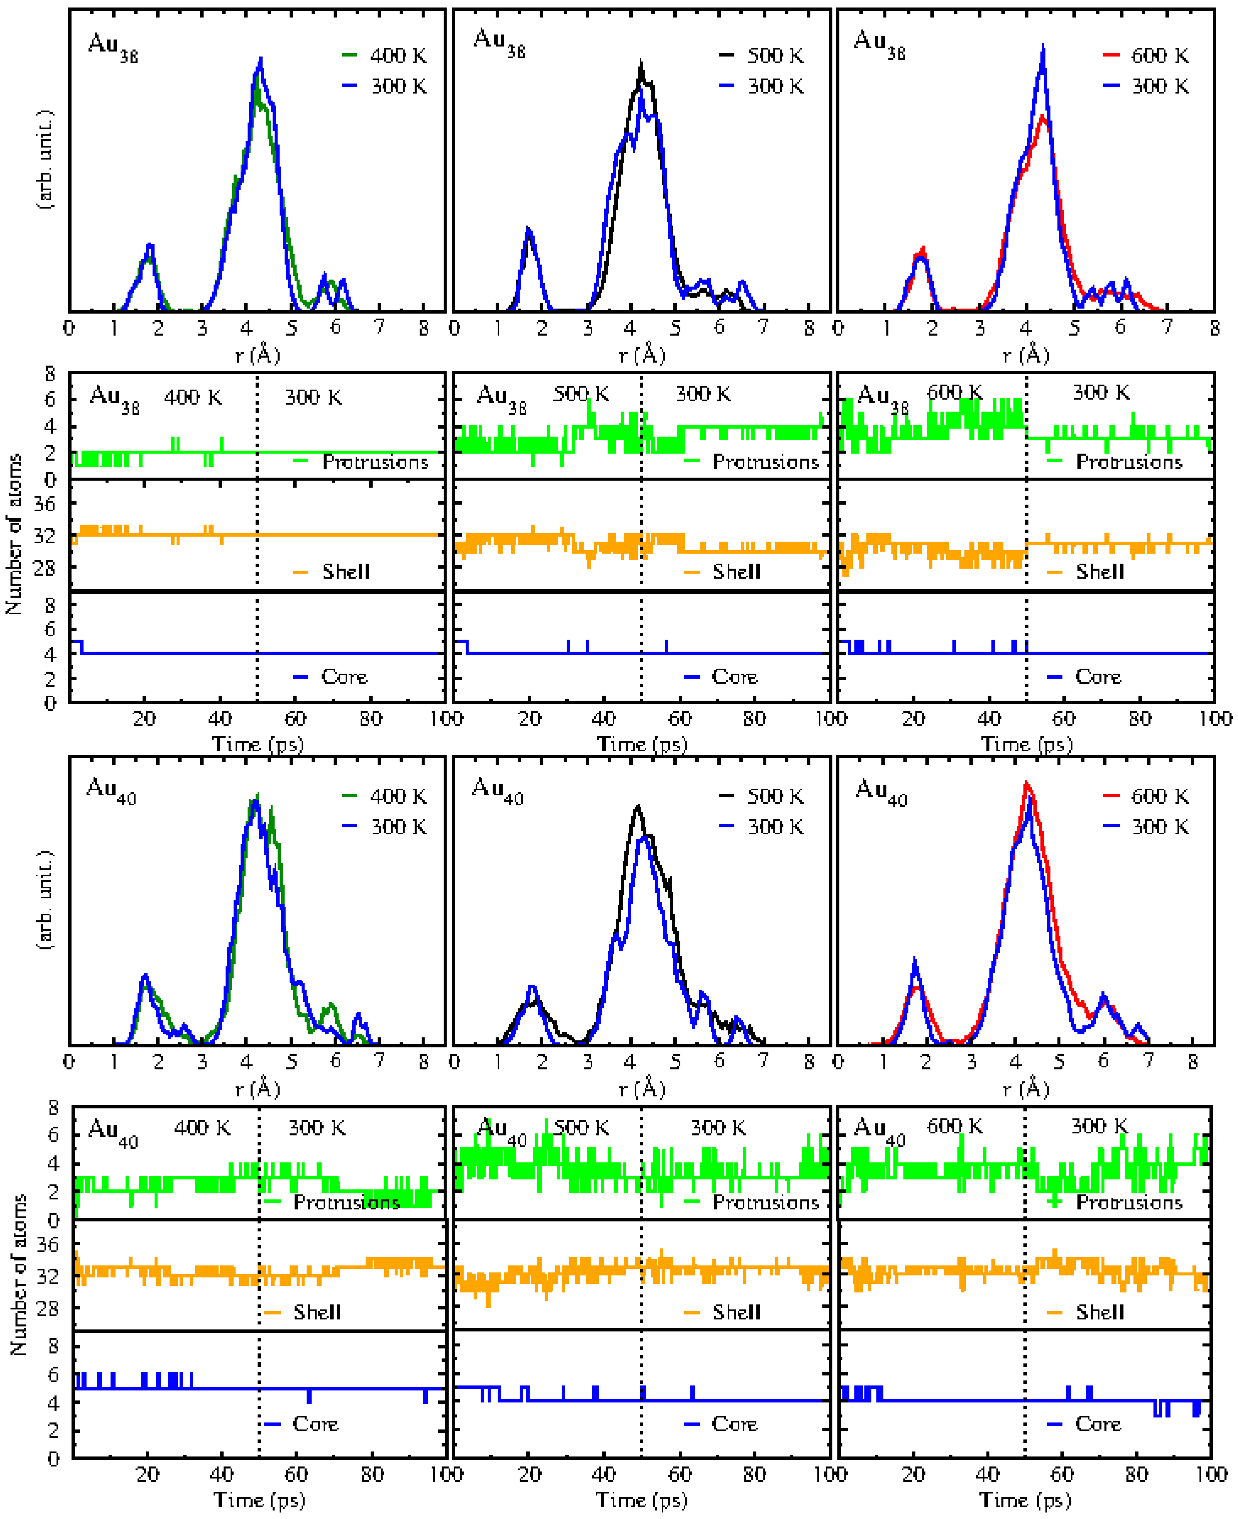


Figure S3 – Radial distribution function, $g(r)$, and number of atoms for core (blue), shell (orange), and protrusions (green), for the MD simulations at 300, 400, 500, and 600 K, starting from $Au_{38}$ and $Au_{40}$ obtained via RBHMC.

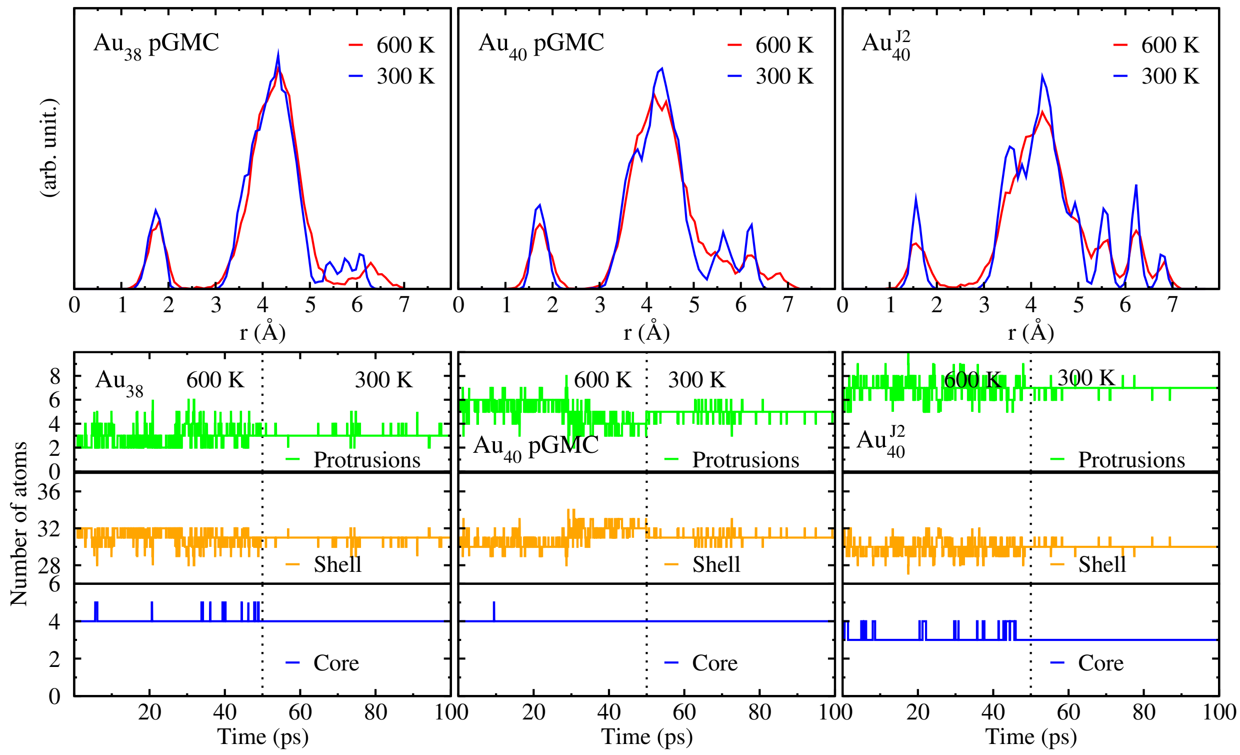


Figure S4 – Radial distribution function, $g(r)$, and number of atoms for core (blue), shell (orange), and protrusions (green), for the MD simulations at 300 and 600 K, starting from $Au_{38}$ and $Au_{40}$ pGMC from Ref. 3.

# II Sketch-map parameters

For $Au_{25}$, the projection with sketch-map was done from of the minimization of the stress function for 500 landmark points randomly selected over all temperatures, by using the sketch-map parameters in $\sigma = 3$, $A = 12$, $B = 4$, $a = 1$, and $b = 2$. For $Au_{38}$ and $Au_{40}$ the sketch-maps projections were created from 500 landmark points randomly selected for both systems over all temperatures. The sketch-map parameters for each were $\sigma = 3.5$, $A = 12$, $B = 10$, $a = 1$, and $b = 2$ for $Au_{38}$, and $\sigma = 3.2$, $A = 12$, $B = 6$, $a = 1$, and 2 for $Au_{40}$. The values of $\sigma$ were chosen to match approximatively the maximum of the pair distribution function in the high-dimensional coordination-histogram representation.

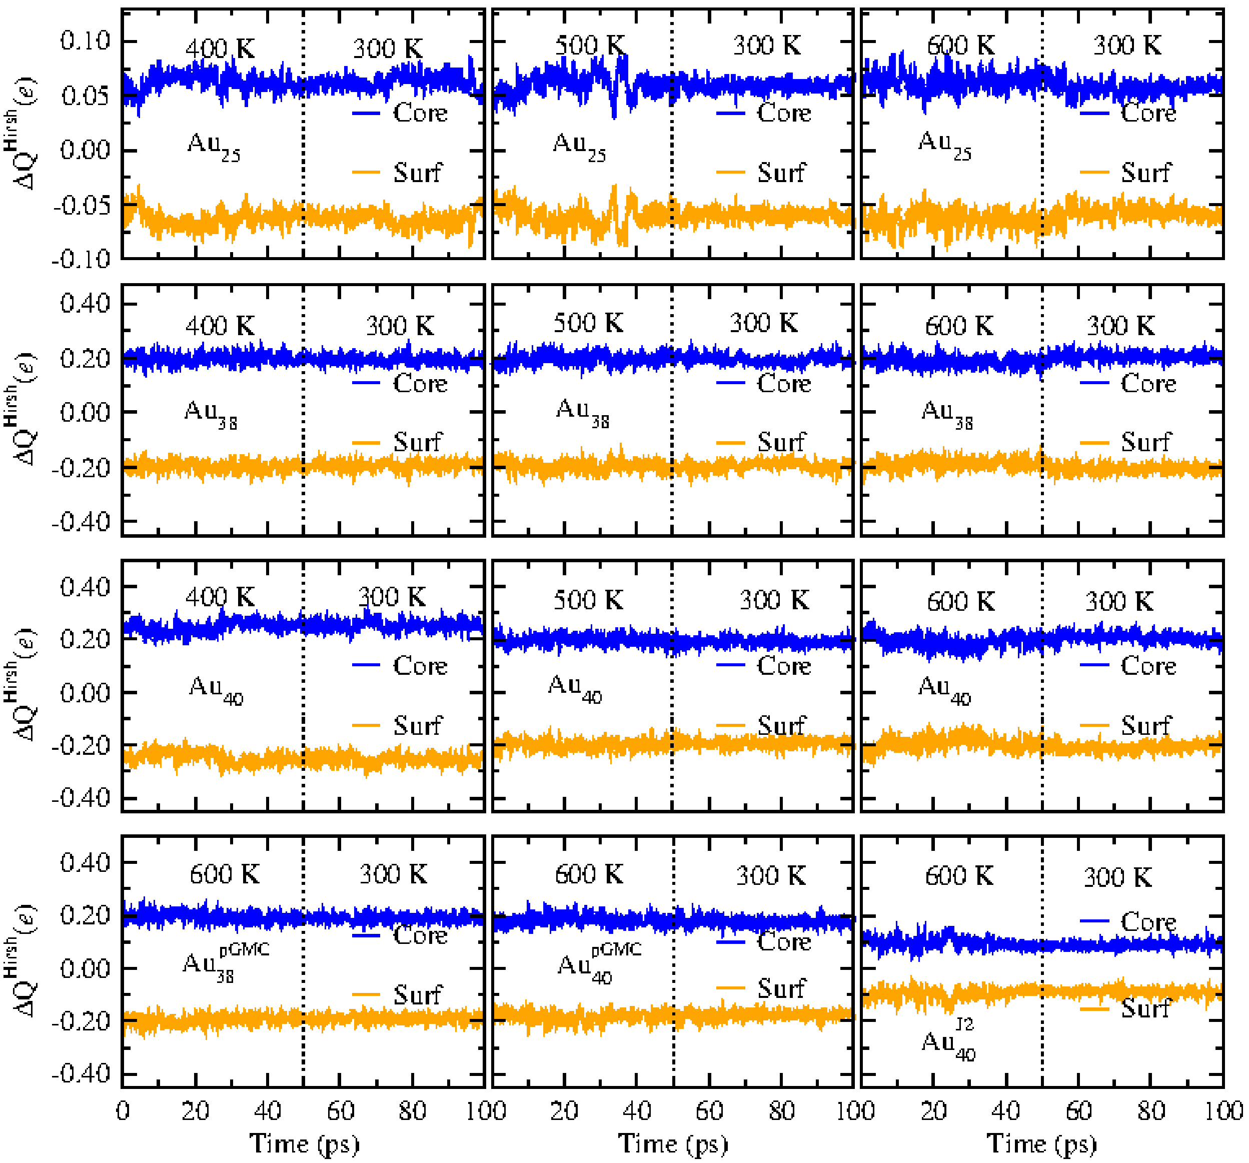


Figure S5 – Total Hirshfeld charge population for surface (orange lines), i.e., shell+protrusions, and core (blue lines) regions at all temperature schemes for $Au_{25}$, $Au_{38}$ and $Au_{40}$ nanoclusters. The sequence of temperatures is indicated for each MD run scheme.

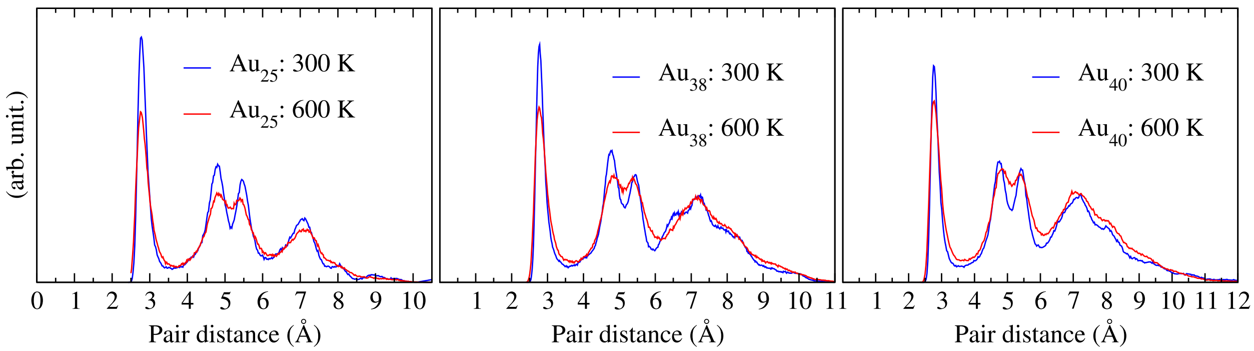


Figure S6 – Pair-distribution function for the $Au_{25}$, $Au_{38}$, and $Au_{40}$ nanoclusters at 300 and 600 K.

**Table S2 – Average bond life time in picoseconds for core-core ($\tau_{cc}$), shell-shell ($\tau_{ss}$), core-shell ($\tau_{cs}$), and shell-protrusions ($\tau_{sp}$) for the $Au_{25}$, $Au_{38}$, and $Au_{40}$ nanoclusters at all temperatures. The bond life time for the pGMC are presented for the MD with $600\,K \rightarrow 300\,K$ temperatures by ${Au_{38}}^{J}$ and ${Au_{40}}^{J_1}$, which correspond to the structures with tetrahedral core with 4 atoms, and ${Au_{40}}^{J_2}$ for the structure with triangular core with 3 atoms. In parentheses are indicated each standard deviation for the bond life times.**

| | $Au_{25}$ – RBHMC | | |
|---|---|---|---|
| | $400\,K \rightarrow 300\,K$ | $500\,K \rightarrow 300\,K$ | $600\,K \rightarrow 300\,K$ |
| $\tau_{ss}$ | 18.06 (6.61) → 20.02 (6.65) | 14.78 (6.07) → 19.31 (6.00) | 10.15 (6.69) → 22.89 (6.96) |
| $\tau_{cs}$ | 14.98 (6.26) → 15.45 (6.34) | 6.02 (4.60) → 15.41 (5.87) | 6.53 (6.35) → 17.75 (7.01) |

| | $Au_{38}$ – RBHMC | | |
|---|---|---|---|
| $\tau_{cc}$ | 22.07 (7.62) → 23.54 (6.78) | 19.76 (7.31) → 22.20 (6.40) | 20.98 (6.30) → 23.80 (0.01) |
| $\tau_{cs}$ | 3.92 (5.26) → 6.47 (5.98) | 2.72 (3.61) → 10.18 (6.53) | 2.40 (4.40) → 7.03 (6.52) |
| $\tau_{ss}$ | 19.58 (6.30) → 21.16 (5.98) | 17.05 (6.45) → 20.35 (6.35) | 15.11 (6.74) → 22.90 (4.99) |
| $\tau_{sp}$ | 17.83 (5.45) → 23.52 (7.71) | 16.27 (4.10) → 20.26 (5.83) | 14.94 (4.23) → 24.29 (7.79) |
| | ${Au_{38}}^{J}$ – pGMC | | |
| $\tau_{cc}$ | | | 15.70 (6.46) → 16.12 (6.75) |
| $\tau_{cs}$ | | | 1.86 (4.37) → 3.36 (6.04) |
| $\tau_{ss}$ | | | 9.09 (6.65) → 9.59 (7.05) |
| $\tau_{sp}$ | | | 7.57 (4.47) → 7.02 (6.88) |

| | $Au_{40}$ – RBHMC | | |
|---|---|---|---|
| $\tau_{cc}$ | 21.54 (7.29) → 22.16 (0.12) | 18.21 (5.96) → 18.87 (6.92) | 15.31 (5.54) → 21.13 (7.26) |
| $\tau_{cs}$ | 7.35 (5.11) → 9.34 (5.98) | 3.06 (3.79) → 5.96 (5.37) | 2.28 (3.09) → 5.89 (5.59) |
| $\tau_{ss}$ | 18.33 (6.35) → 18.81 (5.80) | 14.08 (5.51) → 19.66 (4.56) | 13.26 (5.93) → 20.71 (6.28) |
| $\tau_{sp}$ | 19.33 (6.42) → 25.01 (5.12) | 14.79 (3.24) → 20.42 (6.06) | 10.07 (3.07) → 19.75 (6.79) |
| | ${Au_{40}}^{J_1}$ – pGMC: 4 atoms in the core | | |
| $\tau_{cc}$ | | | 21.80 (7.22) → 24.91 (7.78) |
| $\tau_{cs}$ | | | 2.65 (3.97) → 6.80 (6.93) |
| $\tau_{ss}$ | | | 15.58 (6.03) → 23.65 (6.80) |
| $\tau_{sp}$ | | | 16.42 (4.82) → 23.61 (7.63) |
| | ${Au_{40}}^{J_2}$ – isomer: 3 atoms in the core | | |
| $\tau_{cc}$ | | | 18.46 (4.51) → 23.36 (7.36) |
| $\tau_{cs}$ | | | 3.53 (4.86) → 8.76 (6.59) |
| $\tau_{ss}$ | | | 17.35 (6.28) → 22.68 (6.19) |
| $\tau_{sp}$ | | | 18.65 (6.87) → 23.44 (6.67) |

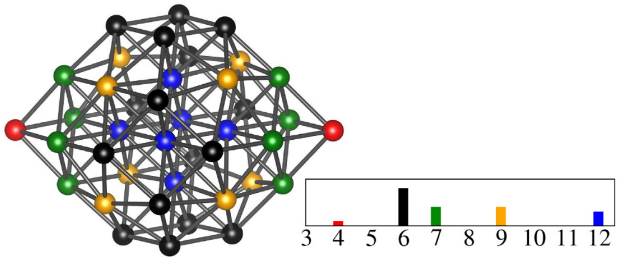


Figure S7 – Histograms of coordination of a $Au_{40}$ nanocluster with truncated-octahedron structure, in which the 4-fold atoms are in red, 6-fold in black, 7-fold in green, 9-fold in yellow, and 12-fold in blue.

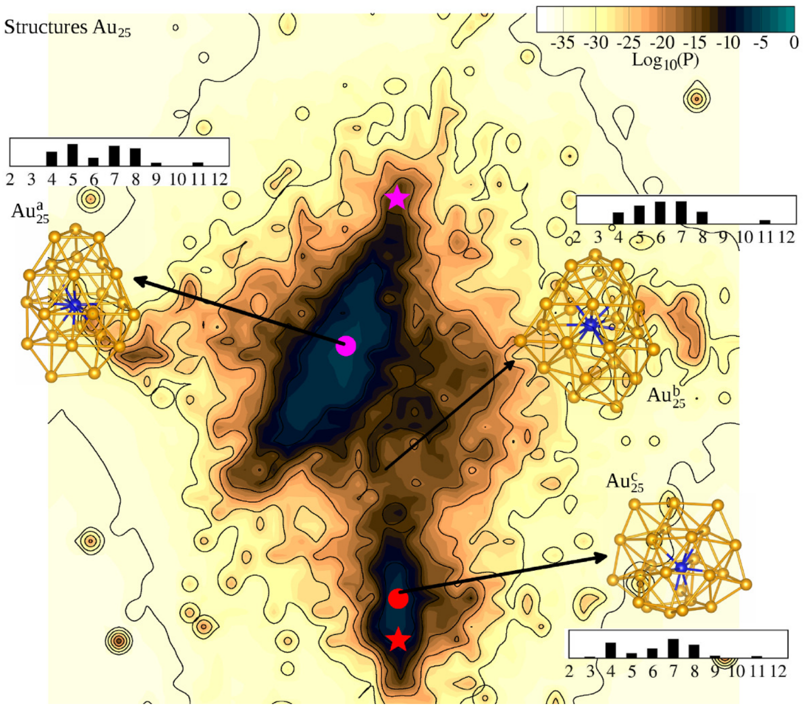


Figure S8 – Probabilities calculated at 300 K via MBAR for all $Au_{25}$ structures sampled all temperatures as a function of the sketch-map coordinates, based on a total 300 ps MD sampling. The represented structures and their respective coordination number histograms were selected from the regions indicated on the sketch-map coordinates. The central atom in each structure is indicated by the blue color, while surface atoms remaining are represented in yellow. Circles and stars with the same color represent initial and final point of geometry relaxations. The pink star is also the pGMC, as found by us.

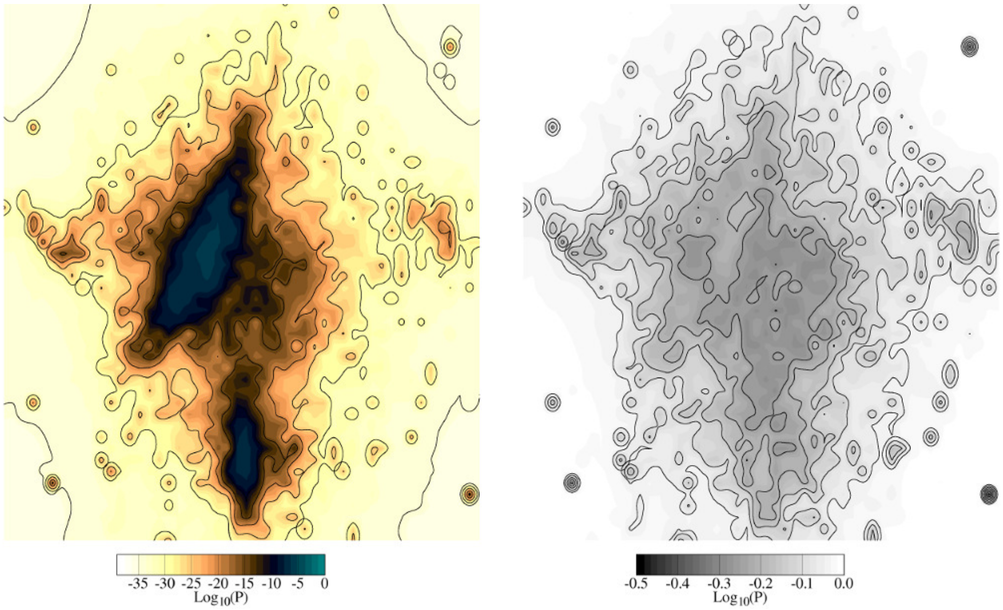


Figure S9 – Probabilities at 300 K calculated via MBAR for all $Au_{25}$ (left side) with error bar (right side) for the structures sampled at all temperatures as a function of the sketch-map coordinates.

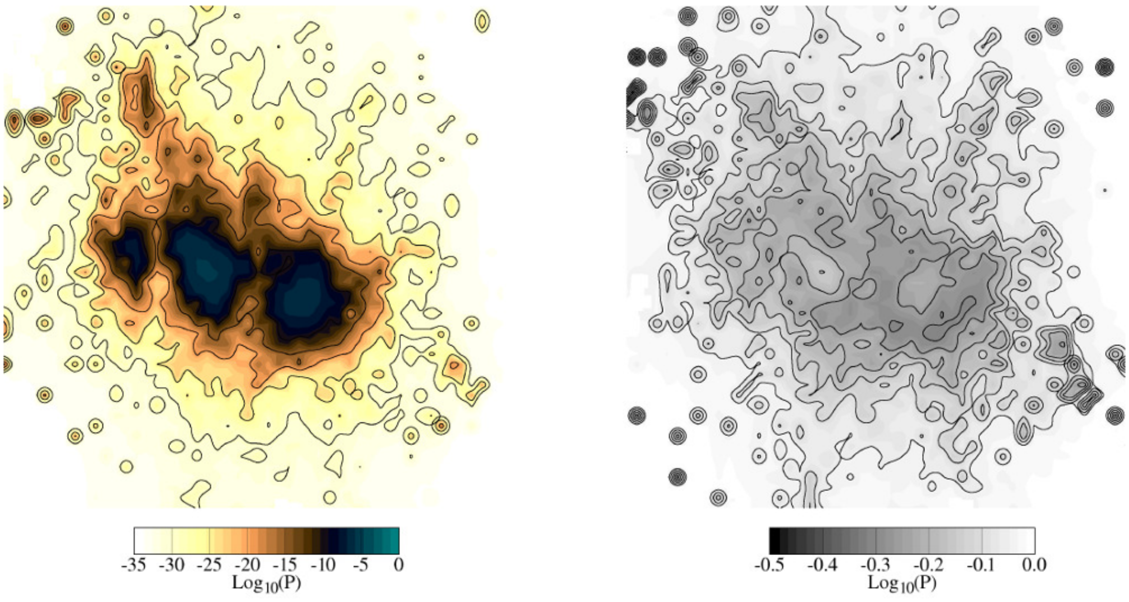


Figure S10 – Probabilities at 300 K calculated via MBAR for all $Au_{38}$ (left side) with error bar (right side) for the structures sampled at all temperatures as a function of the sketch-map coordinates.

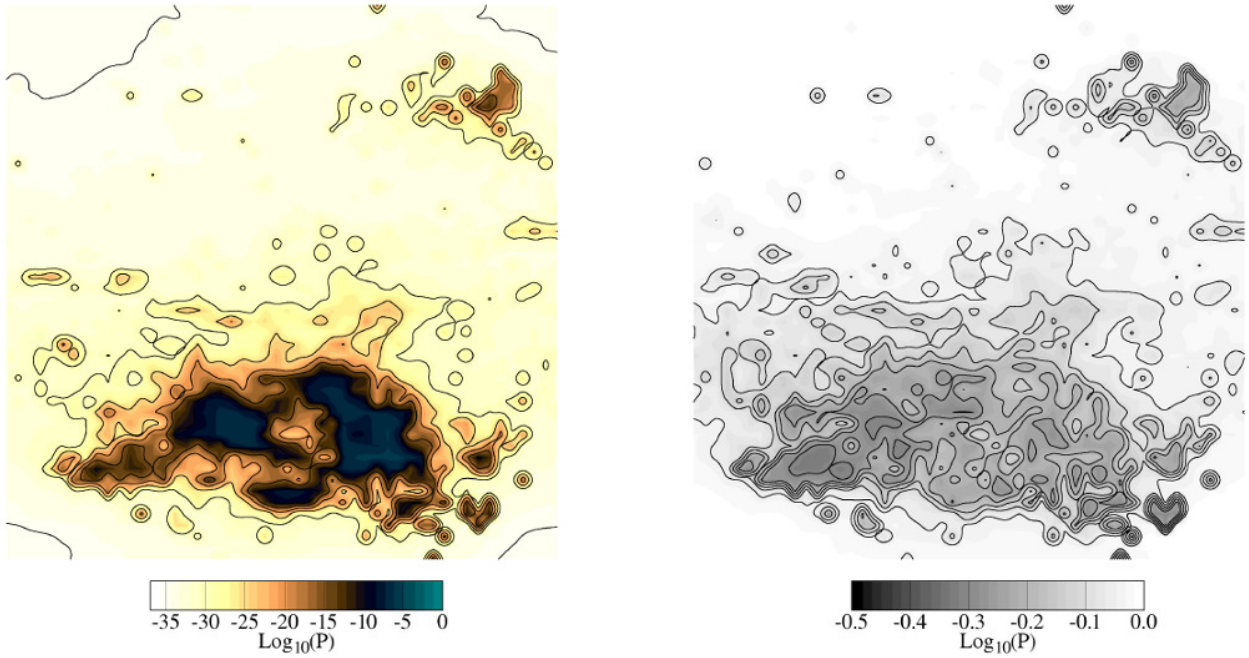


Figure S11 — Probabilities at 300 K calculated via MBAR for all $Au_{40}$ (left side) with error bar (right side) for the structures sampled at all temperatures as a function of the sketch-map coordinates.

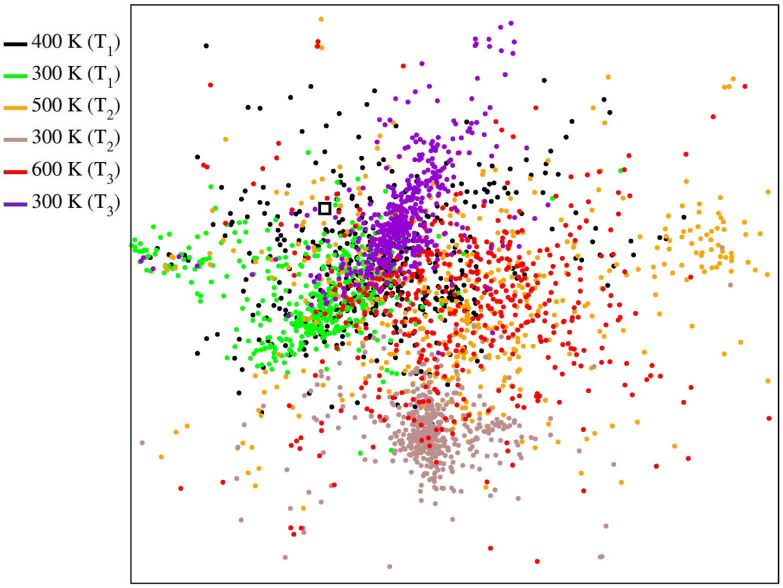


Figure S12 — Sketch-map projection by each 10 MD steps for the $Au_{25}$ structures for all temperatures as summarized at Table 1S. The temperatures are in matching with the Table 1S, from the colours reference as indicated on the labels at $400\,K \rightarrow 300\,K$ of $T_1$ (black and green points), $500\,K \rightarrow 300\,K$ of $T_2$ (orange and brown points), and $600\,K \rightarrow 300\,K$ of $T_3$ (red and violet points). The starting point from the structure obtained via EAM-RBHMC is indicated by the square.

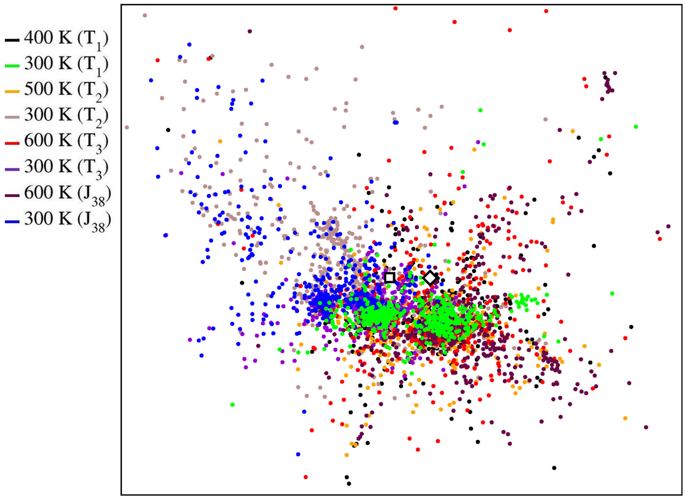


Figure S13 – Sketch-map projection by each 10 MD steps for the $Au_{38}$ structures in each temperature as summarized at Table 1S. The temperatures are in matching with the Table 1S, from the colours reference as indicated on the labels at $400\,\mathrm{K} \rightarrow 300\,\mathrm{K}$ of $T_1$ (black and green points), $500\,\mathrm{K} \rightarrow 300\,\mathrm{K}$ of $T_2$ (orange and brown points), $600\,\mathrm{K} \rightarrow 300\,\mathrm{K}$ of $T_3$ (red and violet points), and $600\,\mathrm{K} \rightarrow 300\,\mathrm{K}$ (marron and blue points) for MD of the Jiang's pGMC for the trajectory $J_{38}$. The starting points from the structures obtained via EAM-RBHMC and pGMC are indicated by the white square and diamond symbols, respectively.

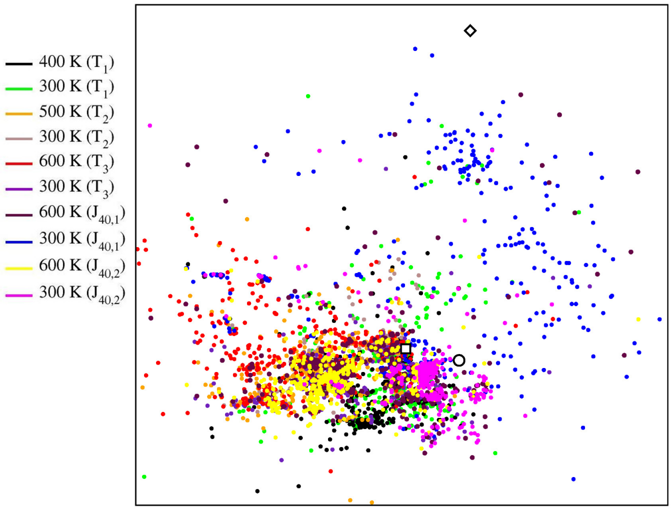


Figure S14 – Sketch-map projection by each 10 MD steps for the $Au_{40}$ structures in each temperature as summarized at Table 1S. The temperatures are in matching with the Table 1S, from the colours reference as indicated on the labels at $400\,\mathrm{K} \rightarrow 300\,\mathrm{K}$ of $T_1$ (black and green points), $500\,\mathrm{K} \rightarrow 300\,\mathrm{K}$ of $T_2$ (orange and brown points), $600\,\mathrm{K} \rightarrow 300\,\mathrm{K}$ of $T_3$ (red and violet points). For the MD of the Jiang's pGMCs for the trajectories, $J_{40,1}$ (with core made by 4 atoms) and $J_{40,2}$ (with core made by 3 atoms), $600\,\mathrm{K} \rightarrow 300\,\mathrm{K}$ (marron and blue points) and $600\,\mathrm{K} \rightarrow 300\,\mathrm{K}$ (yellow and pink points), respectively. The starting points from the structures obtained via EAM-RBHMC, pGMC, and isomer with 3-core atoms are indicated by the white square, circle, and diamond symbols, respectively.

**Table S3** – **Radius of gyration ($R_g$) as defined by $R_g = \sum_i^N s_i/N$ (where $s_i$ is the atom distances from the center of mass and $N$ is the number of atoms), number of core-surface (c-s) bonds, effective coordination number (ECN), and PBE+MBD relative energy for the (unrelaxed) $Au_{25}$, $Au_{38}$, and $Au_{40}$ structures selected from the sketch-map basins and relaxed counterparts. In bold face are the new proposed pGMC for $Au_{25}$ and $Au_{38}$, shown in Fig. S15.**

| | $R_g$ [Å] | # c-s bonds | ECN | Relative Energy [eV] |
|---|---|---|---|---|
| | | | $Au_{25}$ | |
| $Au_{25}^a$ unrelaxed | 17.71 | 13 | 6.01 | 0.751 |
| **$Au_{25}^a$ relaxed** | 17.48 | 14 | 6.31 | **−0.203** |
| $Au_{25}^c$ unrelaxed | 17.56 | 13 | 6.03 | 0.832 |
| $Au_{25}^c$ relaxed | 17.43 | 13 | 6.30 | −0.046 |
| RBHMC relaxed | 17.38 | 12 | 6.30 | 0.000 |
| | | | $Au_{38}$ | |
| $Au_{38}^a$ unrelaxed | 24.93 | 35 | 6.50 | 1.341 |
| **$Au_{38}^a$ relaxed** | 24.82 | 34 | 6.75 | **−0.062** |
| $Au_{38}^b$ unrelaxed | 24.98 | 33 | 6.20 | 2.643 |
| $Au_{38}^b$ relaxed | 24.84 | 34 | 6.61 | 0.203 |
| $Au_{38}^c$ unrelaxed | 25.08 | 35 | 6.19 | 1.880 |
| $Au_{38}^c$ relaxed | 24.91 | 38 | 6.62 | 0.051 |
| $Au_{38}^d$ unrelaxed | 24.95 | 33 | 6.37 | 1.710 |
| $Au_{38}^d$ relaxed | 24.85 | 38 | 6.57 | 0.300 |
| pGMC-Jiang[3] relaxed | 24.76 | 36 | 6.82 | 0.000 |
| RBHMC relaxed | 24.62 | 37 | 6.82 | 0.722 |
| | | | $Au_{40}$ | |
| $Au_{40}^a$ unrelaxed | 26.06 | 33 | 6.51 | 2.001 |
| $Au_{40}^a$ relaxed | 26.13 | 35 | 6.61 | 0.750 |
| $Au_{40}^b$ unrelaxed | 26.05 | 42 | 6.52 | 2.255 |
| $Au_{40}^b$ relaxed | 25.88 | 44 | 6.85 | 0.790 |
| $Au_{40}^c$ unrelaxed | 27.01 | 30 | 6.35 | 1.990 |
| $Au_{40}^c$ relaxed | 26.72 | 30 | 6.55 | 0.265 |
| $Au_{40}^d$ unrelaxed | 26.71 | 36 | 6.26 | 3.104 |
| $Au_{40}^d$ relaxed | 26.22 | 39 | 6.92 | 0.000 |
| $Au_{40}^e$ unrelaxed | 26.30 | 32 | 6.24 | 2.636 |
| $Au_{40}^e$ relaxed | 26.16 | 31 | 6.59 | 0.706 |
| $Au_{40}^f$ unrelaxed | 26.15 | 38 | 6.67 | 1.637 |
| $Au_{40}^f$ relaxed | 26.08 | 38 | 6.91 | 0.198 |
| pGMC-Jiang[3] relaxed | 26.22 | 39 | 6.92 | 0.000 |
| RBHMC relaxed | 25.82 | 39 | 6.85 | 0.897 |

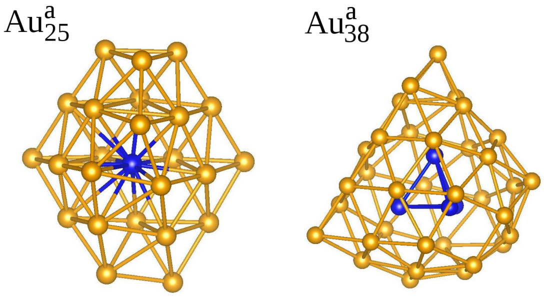


Figure S15 – New pGMC for $Au_{25}$ and $Au_{38}$ obtained from the relaxed MD $Au_{25}{}^{a}$ and $Au_{38}{}^{a}$ configurations, as reported by the relative energies in Table S2.

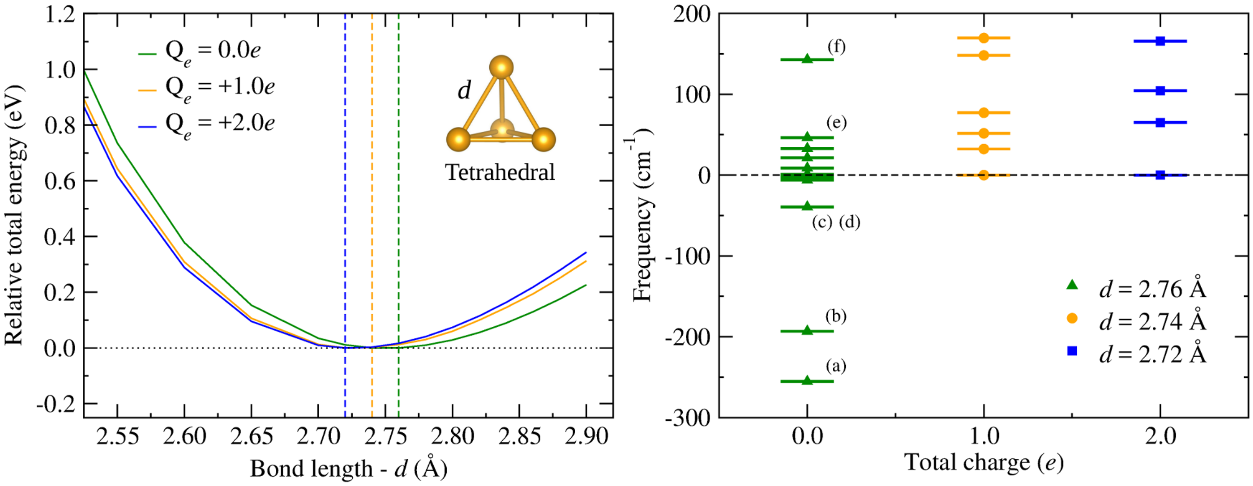


Figure S16 – On the left, relative total energy as a function of the bond length $d$ for the $Au_4$ in tetrahedral configuration for the charge state in $0.0\,e$ (neutral), $1.0\,e$, and $2.0\,e$. On the right, vibrational frequencies for the configurations with lowest energy distance $d$ and charge state in $0.0e$, $+1.0e$, and $+2.0e$. For neutral $Au_4$ tetrahedral, the negative frequencies indicated by (a), (b), (c), and (d) correspond to the vibrational modes, i.e., the neutral tetrahedral configuration is not a local minimum, while for the charge state at $1.0\,e$ and $2.0\,e$ the $Au_4$ tetrahedral is stable.

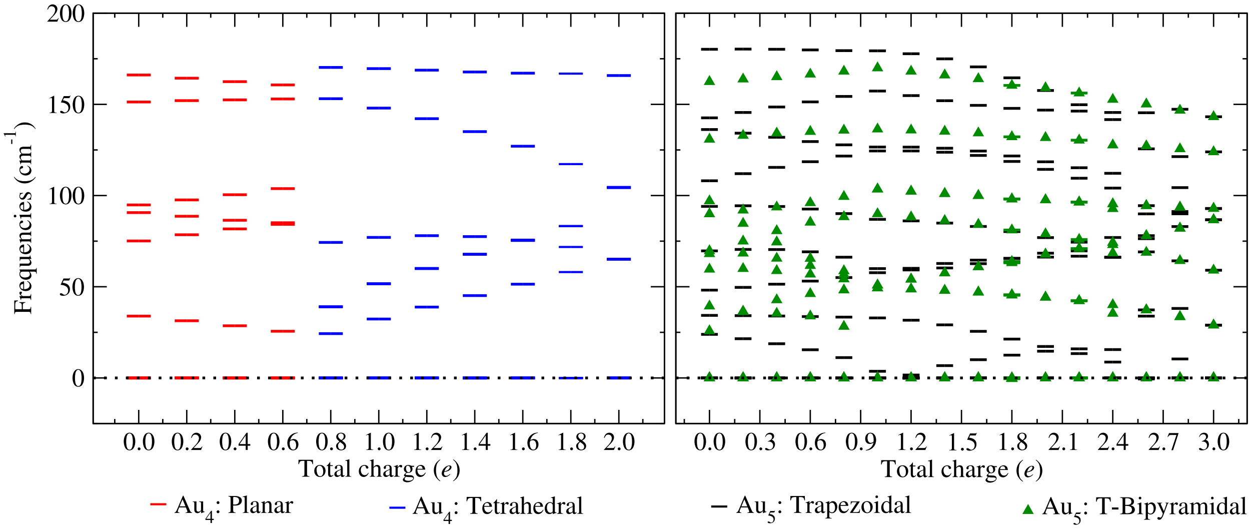


Figure S17 – Vibrational frequencies for the $Au_4$ as planar and tetrahedral and $Au_5$ as trigonal-bipyramidal (T-bipyramidal) configurations relaxed as a function of the positive total charge of the cluster. For $Au_4$ the tetrahedral (blue lines) configuration stabilizes from 0.7$e$ through the relaxation without symmetry constraint via BFGS algorithm. For neutral and positive charges up to 0.6$e$ the structures adopt a perfectly planar configuration or slightly distorted (red lines). For $Au_5$ both trapezoidal and trigonal-bipyramidal are stables for thepositive charges between 0.0 and 3.0$e$.

# References


(1) Blum, V.; Gehrke, R.; Hanke, F.; Havu, P.; Havu, V.; Ren, X.; Reuter, K.; Scheffler, M. Ab Initio Molecular Simulations with Numeric Atom-Centered Orbitals. *Comput. Phys. Commun.* **2009**, *180*, 2175–2196.

(2) Van Lenthe, J. H.; Faas, S.; Snijders, J. G. Gradients in the ab initio scalar zeroth-order regular approximation (ZORA) approach. *Chemical Physics Letters* **2000**, *328*, 107–112.

(3) Jiang, D.; Walter, M. $Au_{40}$: A Large Tetrahedral Magic Cluster. *Phys. Rev. B* **2011**, *84*.

(4) Rondina, G. G.; Da Silva, J. L. F. A Revised Basin-Hopping Monte Carlo Algorithm for Structure Optimization of Clusters and Nanoparticles. *J. Chem. Inf. Model* **2013**, *53*, 2282–2298.
